# Supplementary material for: Context-Aware Group Captioning via Self-Attention and Contrastive Features
Source: arXiv:2004.03708 source file (2020-04-07)
Supplement: Supplementary file 1 [file supp_examples.pdf]

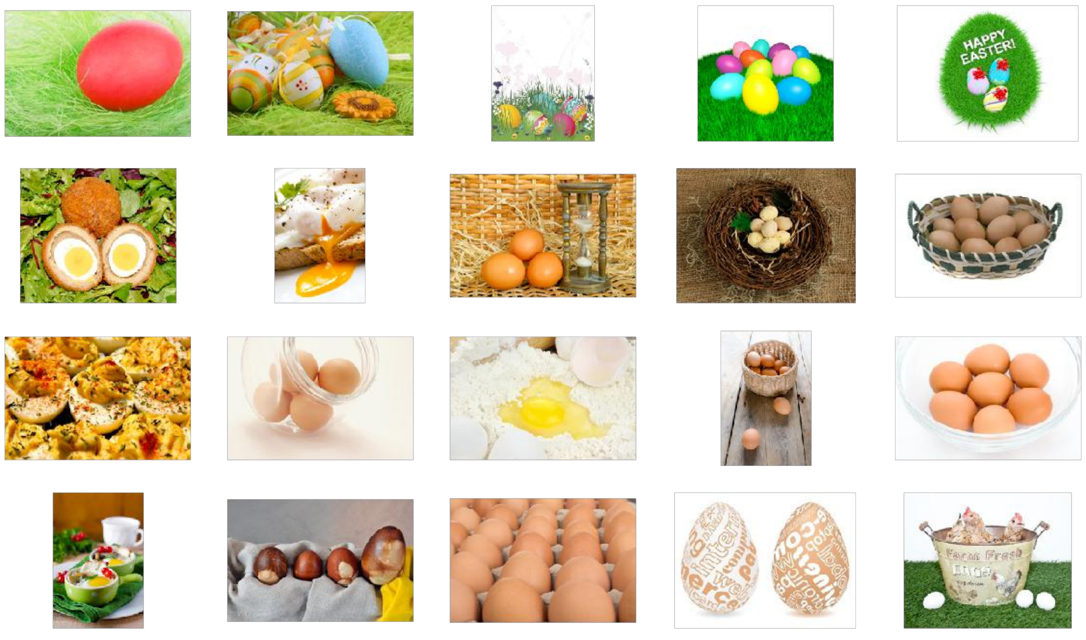


**Ground Truth:** easter eggs on grass
**Our Prediction:** colorful eggs on grass

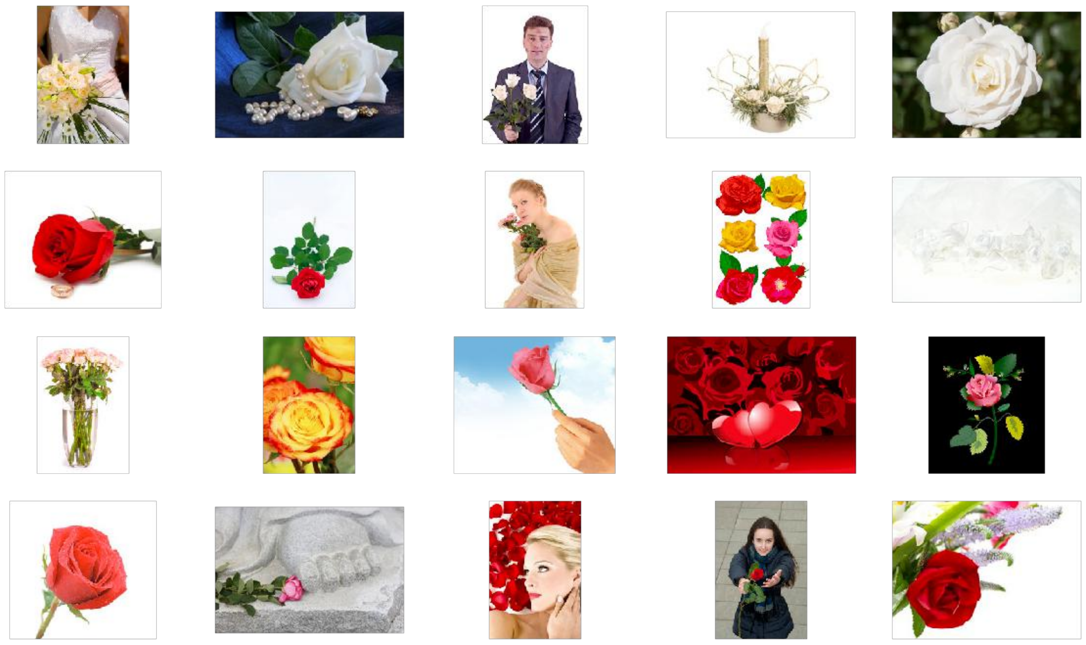

**Ground Truth:** white rose
**Our Prediction:** white rose

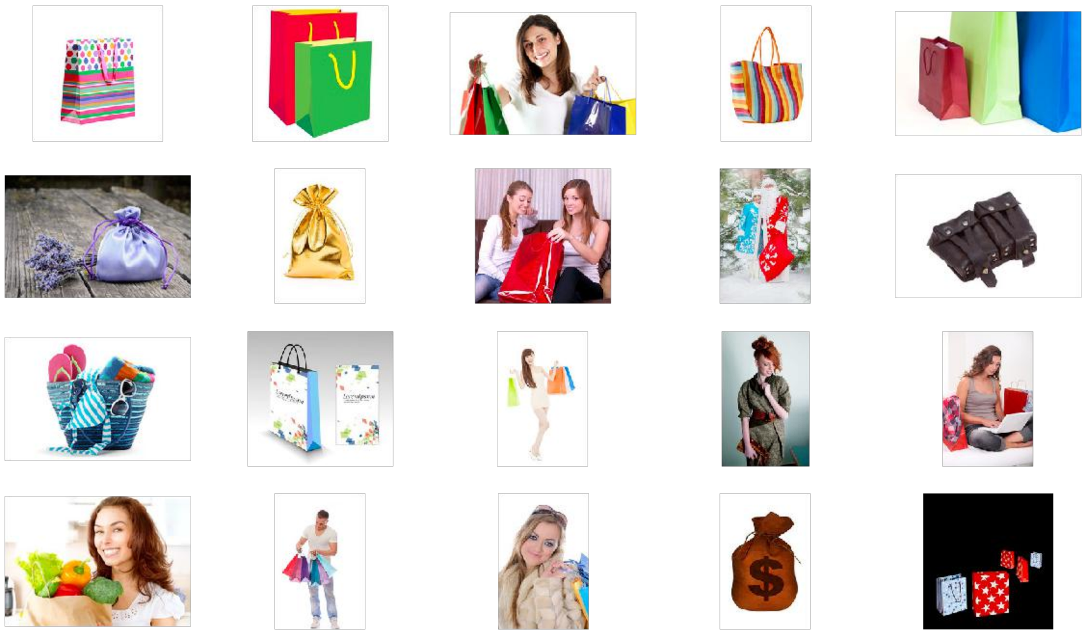

**Ground Truth:** colorful bag on white background
**Our Prediction:** colorful bag on white background

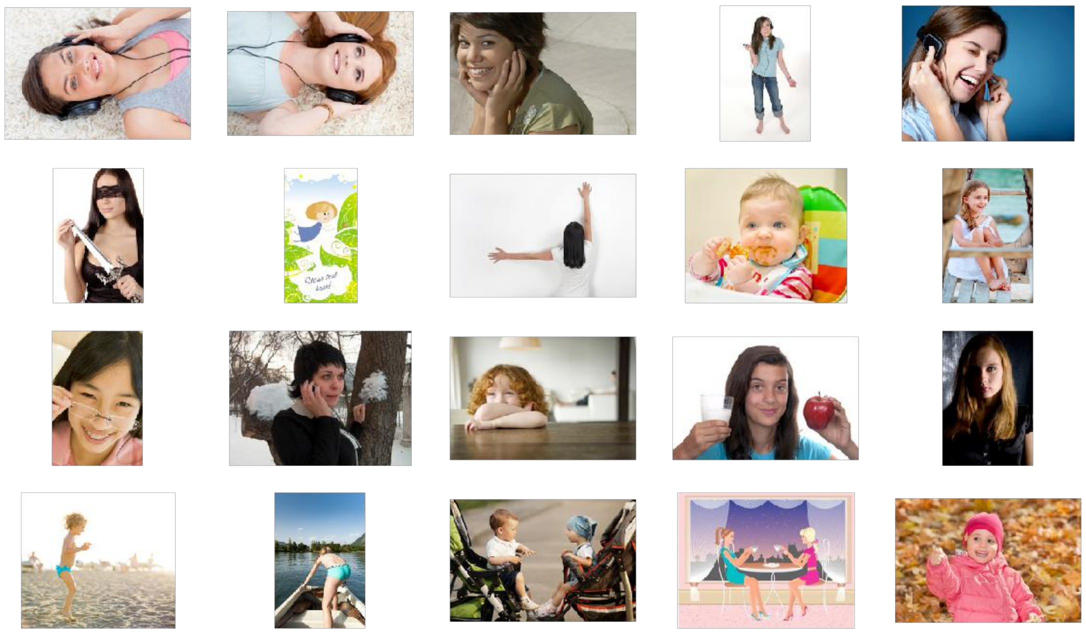

**Ground Truth:** teen girl listening to music
**Our Prediction:** girl listening to music

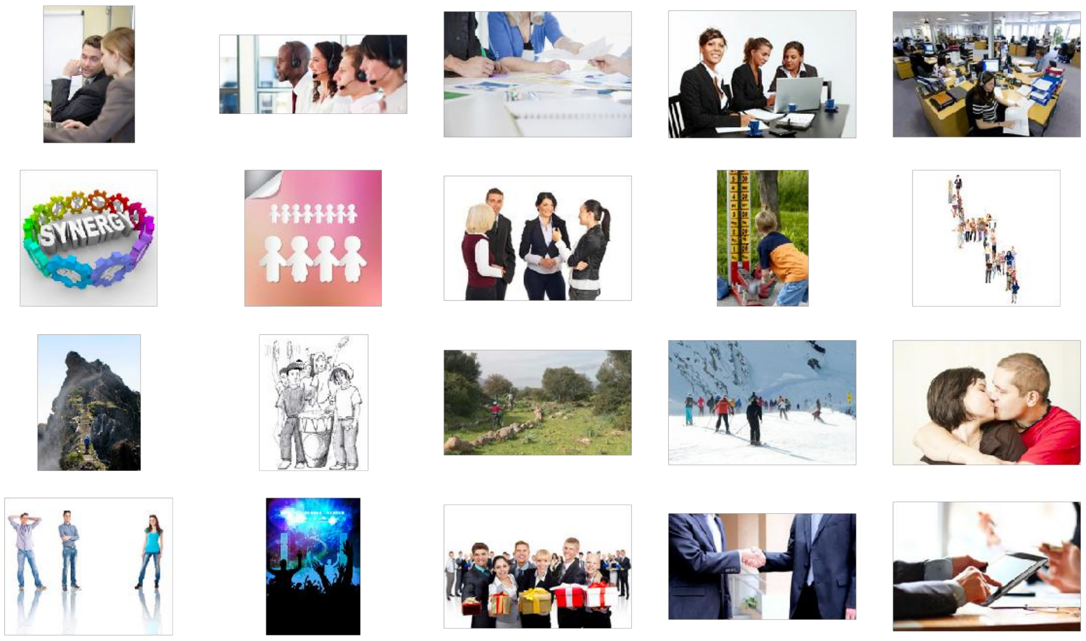

**Ground Truth:** people working in office
**Our Prediction:** business people in office

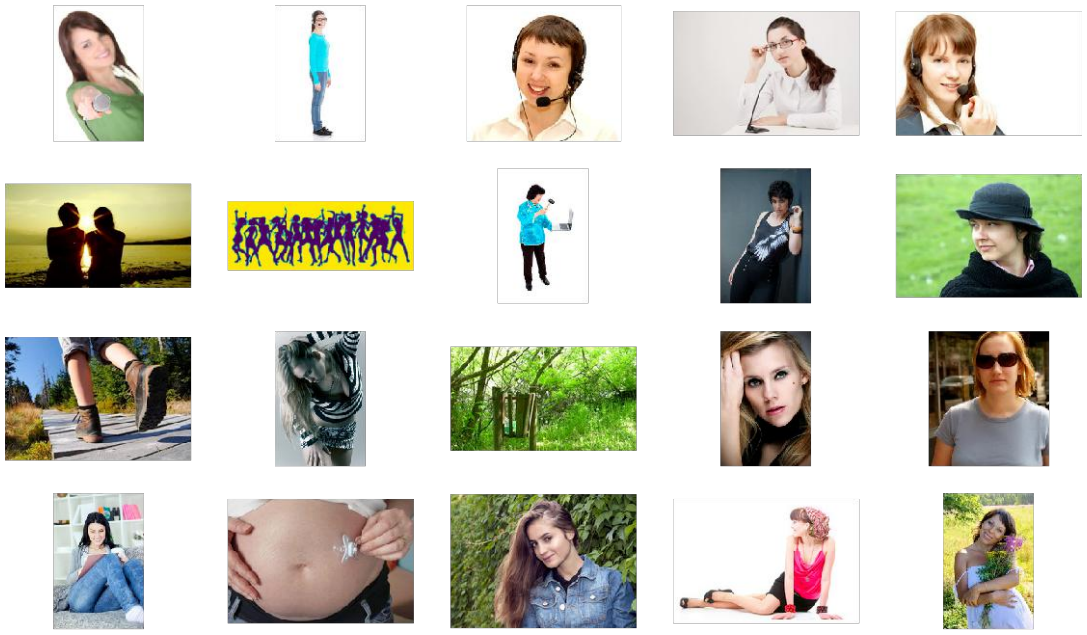

**Ground Truth:** woman with microphone
**Our Prediction:** woman with headset

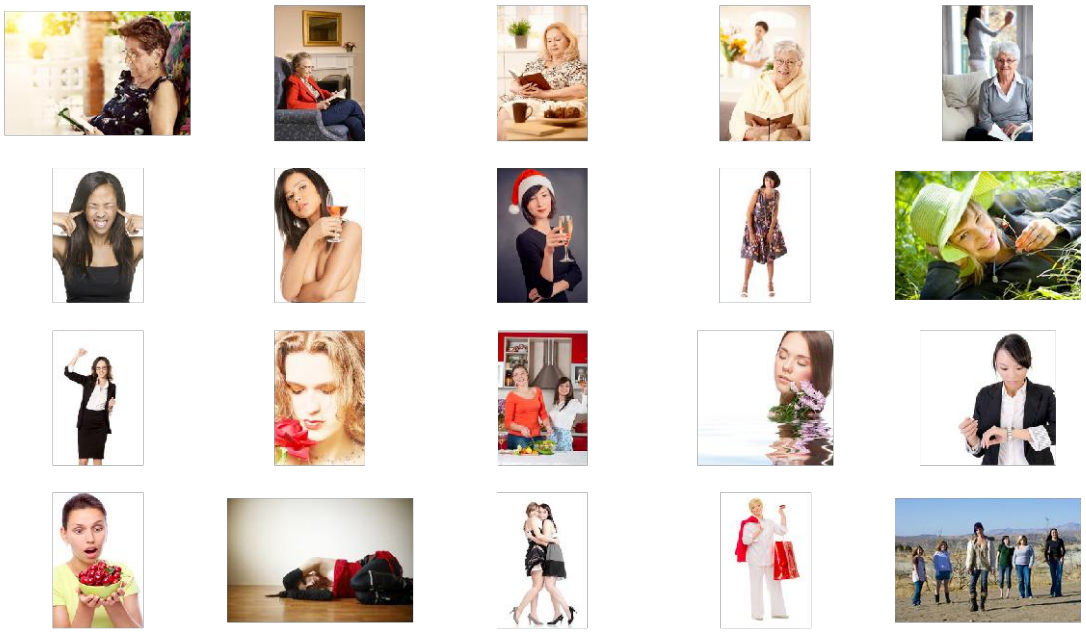

**Ground Truth:** elderly woman reading book
**Our Prediction:** woman reading newspaper

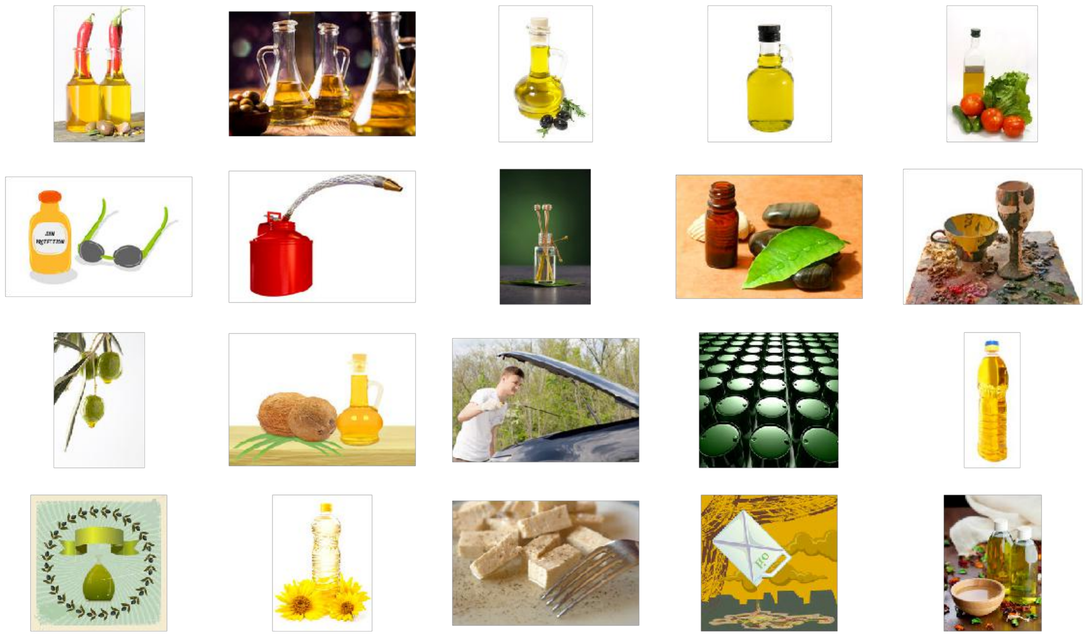

**Ground Truth:** olive oil in bottle
**Our Prediction:** olive oil bottle

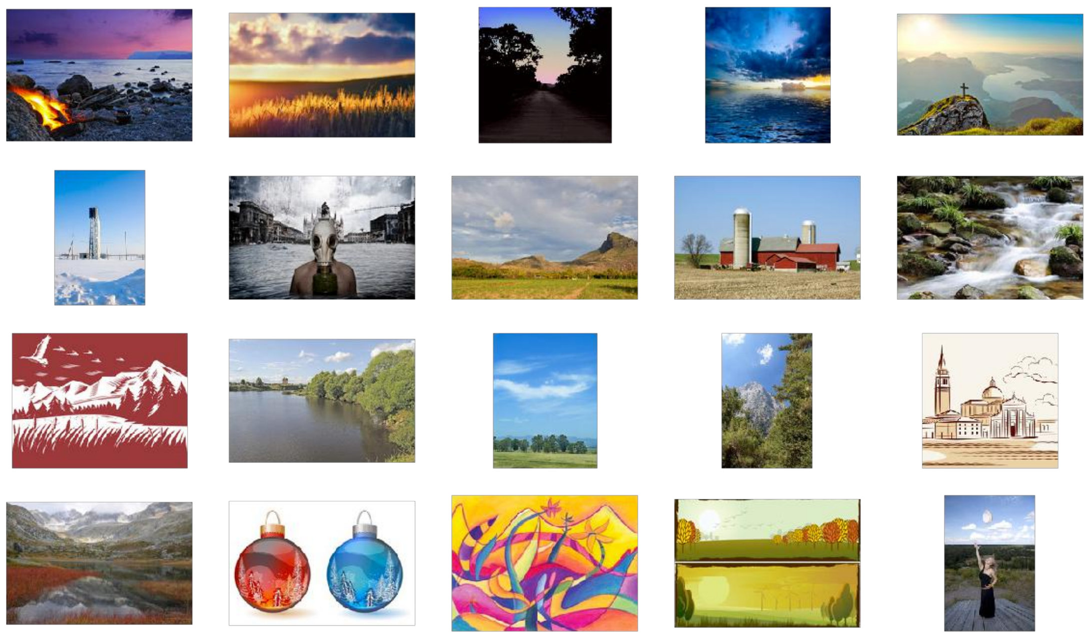

**Ground Truth:** landscape at sunset
**Our Prediction:** sunset landscape

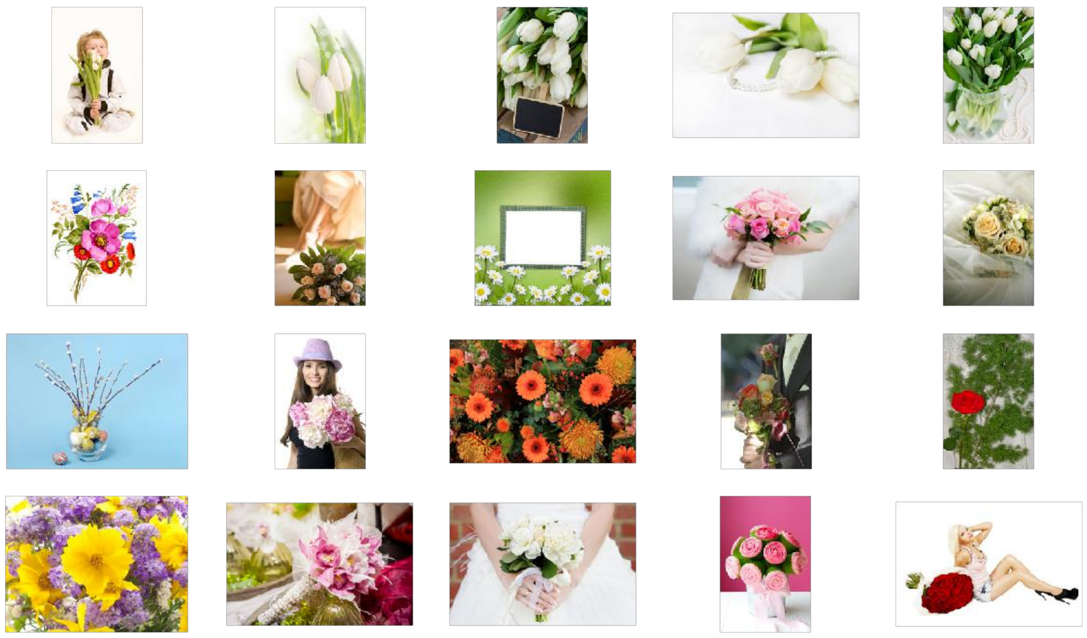

**Ground Truth:** bouquet of white tulip
**Our Prediction:** bouquet of tulip

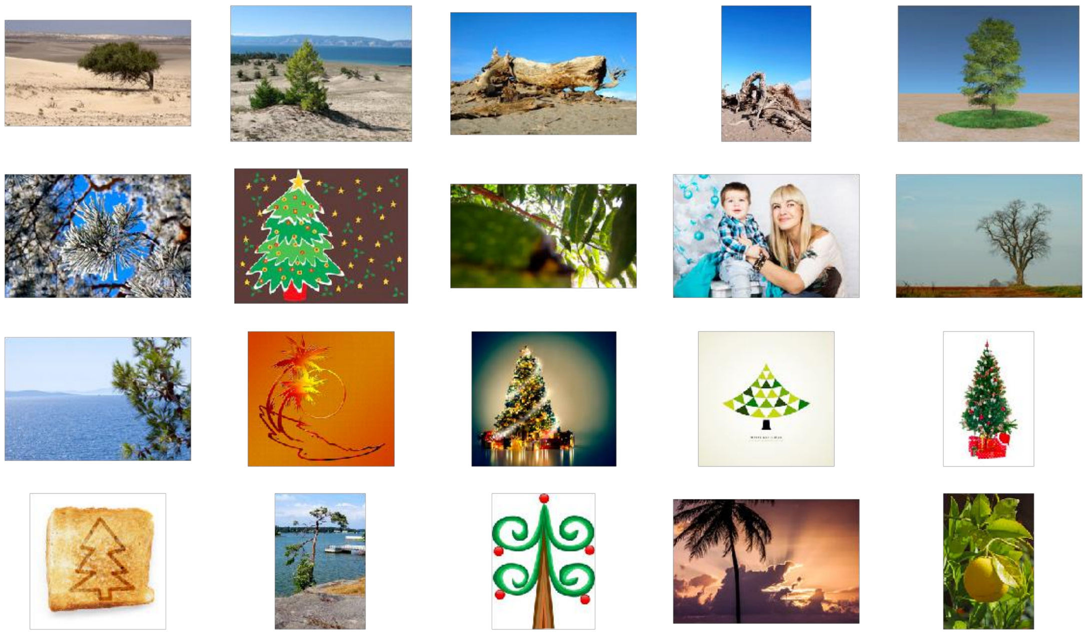

**Ground Truth:** tree in desert
**Our Prediction:** dead tree

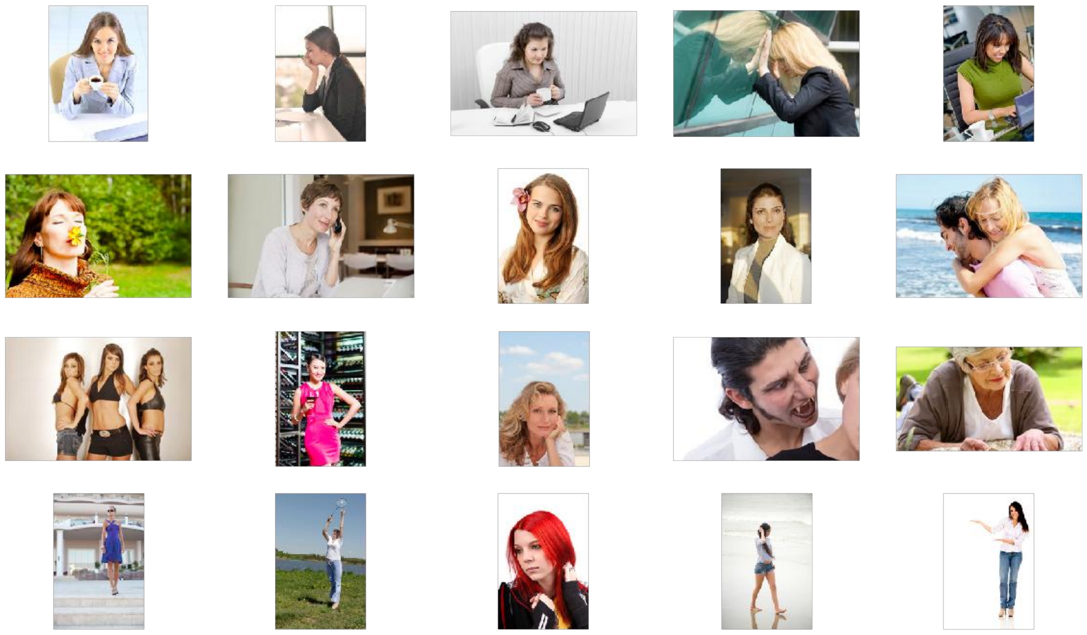

**Ground Truth:** business woman at office
**Our Prediction:** woman using laptop
