# Supplementary material for: Context-Aware Group Captioning via Self-Attention and Contrastive Features
Source: arXiv:2004.03708 source file (2020-04-07)
Supplement: Supplementary file 2 [file supp_failure_case.pdf]

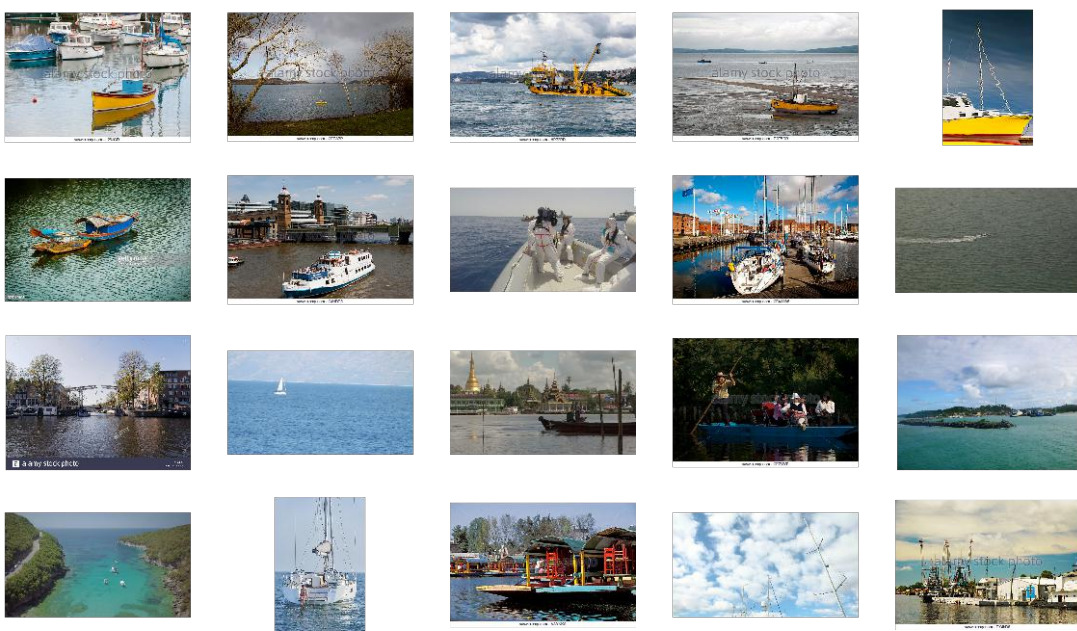

**Ground Truth:** yellow boat

**Our Prediction:** fishing boat

**Group:** boat

**Contrastive:** flaming colorful chart appears colorful  
hypnotic colorful stylized wavy stylized colorful

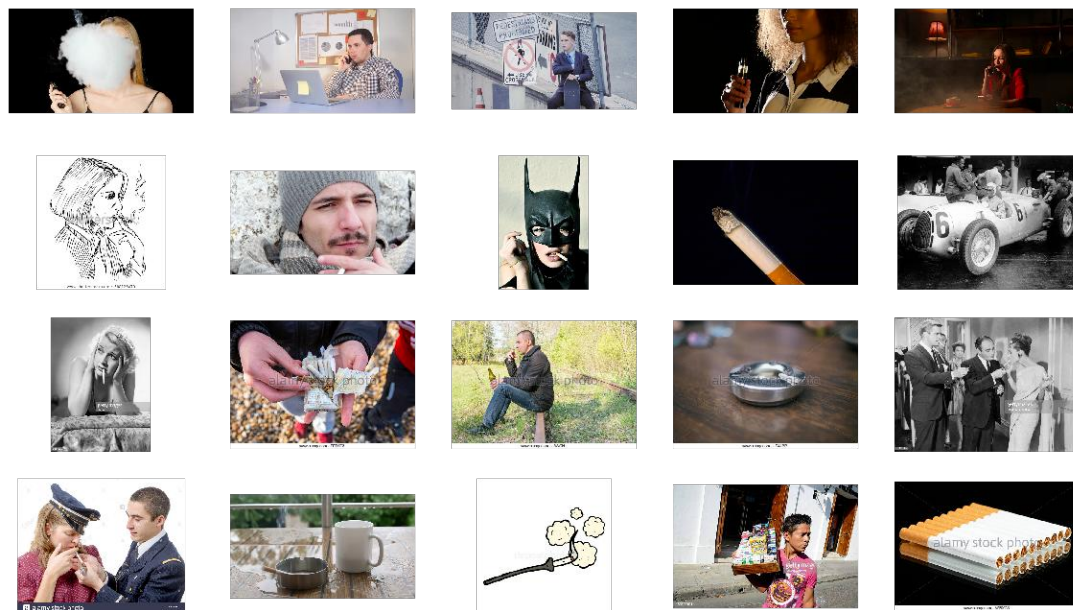

**Ground Truth:** electronic cigarette

**Our Prediction:** white smoke

**Group:** white

**Contrastive:** blue rhythm blue activist on electric  
on pov cigarette call

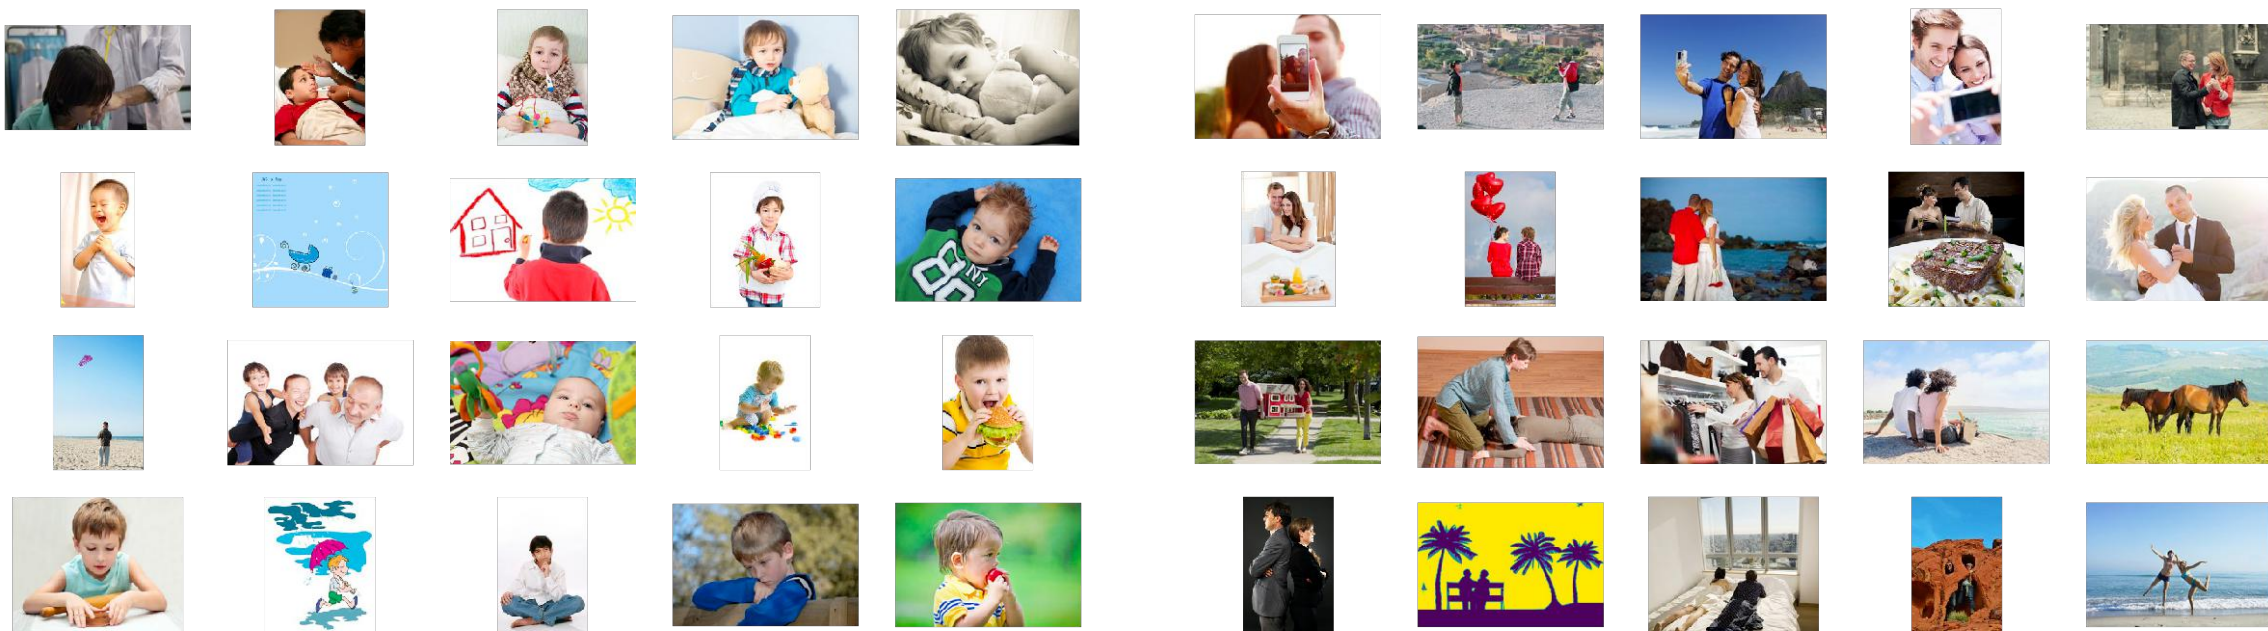

**Ground Truth:** sick boy

**Our Prediction:** boy child

**Group:** boy

**Contrastive:** sick sitting in bed sick bed

**Ground Truth:** couple taking photo

**Our Prediction:** couple using phone

**Group:** couple

**Contrastive:** smile pretty credit mobile using  
mobile phone device
